# Supplementary material for: Multi-Sensor Fusion of Active and Passive Measurements for Extended Object Tracking
Source: arXiv:2504.18301 source file (2025-04-25)
Supplement: Supplementary file 1 [file appendix.tex]

% placeholder for appendix
% dont think there will be one
% maybe further work?

\section{Derivation of the data association prior}

lalalalal
